# Supplementary material for: Hypergraph Multi-modal Large Language Model: Exploiting EEG and Eye-tracking Modalities to Evaluate Heterogeneous Responses for Video Understanding
Source: arXiv:2407.08150 source file (2024-09-05)
Supplement: Supplementary file 1 [file figure-appendix-con-0412.pdf]

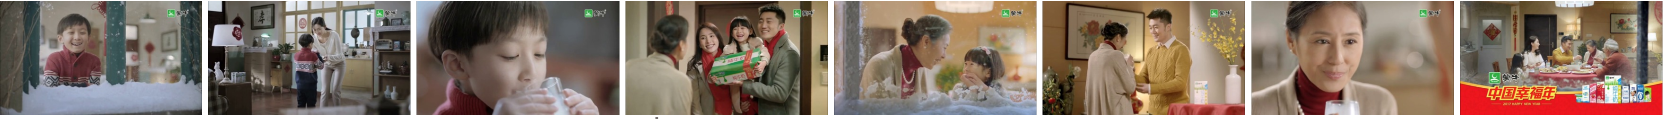

**Question**: What does this video describe overall?

This video usually appears in the context of family and warm atmosphere, and may describe a warm scene of a family during winter, especially during **new years or holidays**. The video may showcase emotional communication among family members, such as the interaction between children and parents, grandmother and granddaughter, and the happy moments of family gatherings. The presentation of the product (possibly **milk or dairy products**) indicates that the video may be a **commercial advertisement** aimed at conveying the connection between the product and family health and happiness. The tail of the video may display the product brand and New Year's greetings, giving people a warm and peaceful feeling. The entire video may emphasize the warmth of family reunion and the joy of holiday moments.

Gemini: This video shows a young boy looking out his window at the snow falling. He is smiling and appears to be happy. The video is set in a rural area, and the boy is wearing a traditional Chinese outfit. The video is likely intended to **evoke a sense of nostalgia and happiness**.

Video-LLaVA: This video showcases a family enjoying **a snowy** day together, with scenes of a boy drinking **milk**, a woman drinking from a carton, and a man and woman drinking from a glass. The video also features a family enjoying a meal together at a table.

VideoChat2: This video depicts a **celebration** of a holiday.

HMLLM: This video looks like a **commercial advertisement**. The video may showcase different scenes of a family enjoying **milk**, emphasizing the importance of milk in family life and the joy of family gatherings. The video may also include scenes of family members celebrating holidays or special occasions, such as the **New Year**, and may include product displays and brand information. Overall, the video aims to convey the **warmth** of family, the joy of holiday celebrations, and the role of milk in enhancing these beautiful moments.

**Question**: Please assess the engagement indicator after watching the video.

Engagement: cognitive

Gemini: Engagement: cognitive
Video-LLaVA: Engagement: non-cognitive
VideoChat2: Engagement: cognitive
HMLLM: Engagement: cognitive

**Question**: If you are **a male aged 36 to 40**, how would your EMR duration change after watching this video?

EMR duration: fully attended

Gemini: EMR duration: partially attended
Video-LLaVA: EMR duration: partially attended
VideoChat2: EMR duration: fully attended
HMLLM: EMR duration: fully attended

**Question**: After watching the video, what sort of trend may emerge in a **31 to 35-year-old woman's** EMR duration?

EMR duration: partially attended

Gemini: EMR duration: partially attended
Video-LLaVA: EMR duration: partially attended
VideoChat2: EMR duration: fully attended
HMLLM: EMR duration: partially attended

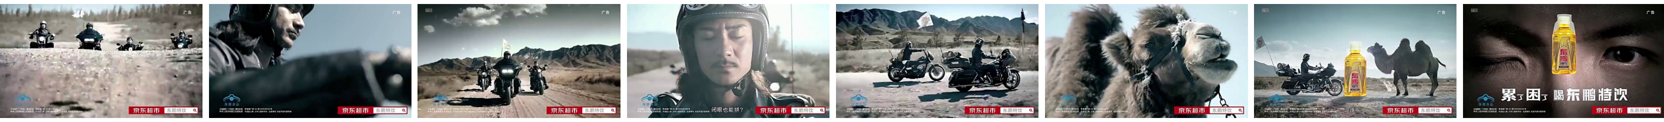

**Question**: What is the main audience for this video advertisement?

This video seems to be an **advertisement** that uses a comparison between a motorcycle rider and a desert camel, as well as some dramatic filming techniques, to attract the audience's attention. The motorcycle rider in the video seems to be exploring and traveling in a harsh desert environment. Finally, the advertisement showcases the product - a bottle of **functional beverage**, combined with slogans and visual elements - to convey that the product can enhance the endurance and physical function of motorcycle riders in extreme challenging environments, supporting users to achieve better results. Overall, this advertisement aims to showcase the advantages and characteristics of its product by highlighting themes of **adventure and endurance**.

Gemini: Based on the video's dimensions, the main audience for this video advertisement is likely to be people who are **interested in traveling to or learning about the Gobi Desert**. The video is shot in a documentary style, and it provides a lot of information about the camels and the people who live in the desert. The video is also very visually appealing, and it is likely to make viewers want to learn more about the Gobi Desert.

Video-LLaVA: The main audience for this video advertisement is likely people who enjoy adventure and exploration, as well as those who appreciate the beauty of nature and the thrill of **traveling on a motorcycle**. The video showcases the excitement and freedom of exploring the world on a motorcycle, and the adrenaline rush of traveling through different terrains.

VideoChat2: The primary target audience for this advertisement is the Chinese audience.

HMLLM: This video advertisement is mainly aimed at outdoor adventure enthusiasts. The video shows a motorcycle rider and a camel, as well as a close-up of a bottle of product, which may be a **beverage or energy drink**. The video may emphasize the **vitality and adventure** of the product, and may be promoting a certain energy drink or other beverage that can provide energy or is related to motorcycle riding. The video may also emphasize the connection between the product and the lifestyle of motorcycle riders, aiming to attract this target audience.

**Question**: In terms of 31 to 35-year-old women, what is the typical performance they exhibit in the area of emotion post-video viewing?

emotion: neutral

Gemini: emotion: neutral
Video-LLaVA: emotion: neutral
VideoChat2: emotion: positive
HMLLM: emotion: neutral

Gemini Gemini-Pro-vision | Video-LLaVA | VideoChat2 | HMLLM(ours)

A). Ground Truth

B). Inference by Different Models

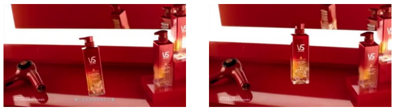

**Question**: What does this storyboard describe?

This storyboard showcases a **shampoo** and **hair care product**, creating an atmosphere of a professional hair salon. The background is red, conveying the passion or high-end brand image of the product. You can also see a professional **hair dryer**, which enhances the connection between the product and professional hair care and styling. The overall storyboard emphasizes the professionalism of the product and its role in hair care.

A). Ground Truth

Gemini: The storyboard describes a commercial for a line of hair care products. The video will feature a woman with long, damaged hair. She will be shown using the products to wash, condition, and style her hair. The final shot will show her with healthy, shiny hair.

This storyboard describes a bottle of red liquid on a red background, with a red and white label. The liquid is shown being poured into a glass and being sprayed on a person's face.

The storyboard depicts the use of a shower gel.

This storyboard showcases a series of hair care products, mainly shampoo and conditioner, placed in a bright and red toned environment. The entire scene is designed to highlight the product's design and color, conveying a high-end and professional hair care brand image. The video may be an advertisement for the brand, aimed at attracting audience interest in the product and encouraging them to purchase.

B). Inference by Different Models
